# Supplementary material for: Full-field hard x-ray microscopy with interdigitated silicon lenses
Source: arXiv:1506.06677 source file (2015-06-22)
Supplement: Supplementary file 1 [file supp_mater.pdf]

## SUPPLEMENTARY MATERIAL

### Full-field hard x-ray microscopy with interdigitated silicon lenses

Hugh Simons,[1,2,a)] Frederik Stöhr,[3] Jonas Michael-Lindhard,[3] Flemming Jensen,[3] Ole Hansen,[4,5] Carsten Detlefs,[2] and Henning Friis Poulsen[1]

[1)] *Department of Physics, Technical University of Denmark, Building 307, Kgs. Lyngby DK-2800, Denmark*

[2)] *European Synchrotron Radiation Facility, Grenoble 38000, France*

[3)] *DANCHIP, Technical University of Denmark, Building 347, Kgs. Lyngby DK-2800, Denmark*

[4)] *DTU Nanotech, Technical University of Denmark, Building 345E, Kgs. Lyngby DK-2800, Denmark*

[5)] *CINF, Technical University of Denmark, Building 345E, Kgs. Lyngby DK-2800, Denmark*

(Dated: 28 April 2015)

[a)] Electronic mail: husimo@fysik.dtu.dk

# I. FORMALISM

## A. Underlying assumptions

This formalism describes the optical properties of absorption-limited compound refractive x-ray lenses (CRLs) and their role as objectives in full-field x-ray microscopes (XRMs). It makes extensive use of ray transfer matrix (RTM) analysis; a geometrical method of calculating the position and angle of a ray after simple optical processes such as propagation, reflection and refraction[1]. When used to simulate CRLs[2–5], this approach has the key advantage that the cumulative effects of many individual optical processes (e.g. many lenslets) can be described as a single $2 \times 2$ transfer matrix $\mathbf{M}$ that acts upon a ray of position $r_0$ and angle $w_0$ to give it a new position $r_1$ and angle $w_1$:

$$\begin{bmatrix} r_1 \\ w_1 \end{bmatrix} = \mathbf{M} \begin{bmatrix} r_0 \\ w_0 \end{bmatrix} \tag{1}$$

However, the RTM approach makes a number of assumptions that should be kept in mind:

1. *Paraxial rays*: Inherent to the RTM method is the paraxial approximation that the angle between all geometrical rays and the optical axis are small such that $\sin w \approx w$ and $\cos w \approx 1$. This approximation is justified by the weak refractive decrement $\delta$ and small aperture of x-ray CRLs.

2. *Thin lens approximation*: The focal length of a single element is much larger than its thickness (e.g. a single Si lenslet with a 20 $\mu$m radius of curvature will have a thickness in the order of 0.5mm but a focal length of nearly 5m at 15 keV). The thin lens approximation has been shown to be valid for the vast majority of lens geometries[5] and simplifies analysis considerably.

3. *Absorption-limited aperture*: This approximation is not always justified for CRLs comprising only a few lenslets of low-absorbing material (e.g. Be). However, for the specific applications under consideration here (short focal lengths and many lenslets with non-neglible absorption), the field strength outside of the geometrical aperture is inconsequential. Also note that this assumption negates the effects of separation between lenslets.

4. *No internal reflection*: The lenslets would be impractically long before the parabolic sidewalls were sufficiently steep to approach the critical angle for reflection at hard energies[4].

5. *No diffraction*: Such effects cannot be explicitly accounted for by geometrical approaches, but are considered later in the estimation of optical performance.

## B. Focusing

We first consider the simplest one dimensional (1D) lenslet geometry of a planar or axisymmetric CRL comprising $N$ lenslets, each with refractive decrement $\delta$ and a parabolic profile defined by an apex radius of curvature of $R$, lenslet thickness of $T$ (i.e. spacing between adjacent lenslet centers) and web thickness between apices of $T_0$ (See Fig. S1).

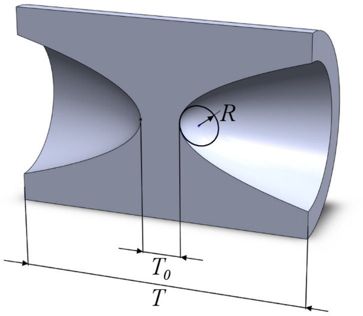


FIG. S1. Geometry of the 1D radially symmetric (i.e. axisymmetric) refractive lenslet

Assuming thin lens behaviour (i.e. $f \gg T$), the focal length of the individual lenslets is[6]:

$$f = \frac{R}{2\delta} \tag{2}$$

With the RTM approach, the transfer matrix $\mathbf{M}$ of the individual lenslet is then given as a free space propagation by half the lenslet thickness ($T/2$), followed by focusing by a thin lens with focal length $f$ and another free space propagation by $T/2$:

$$\mathbf{M} = \begin{bmatrix} 1 & T/2 \\ 0 & 1 \end{bmatrix} \begin{bmatrix} 1 & 0 \\ -1/f & 1 \end{bmatrix} \begin{bmatrix} 1 & T/2 \\ 0 & 1 \end{bmatrix} = \begin{bmatrix} 1 - \frac{T}{2f} & T - \frac{T^2}{4f} \\ \frac{-1}{f} & 1 - \frac{T}{2f} \end{bmatrix} \tag{3}$$

The cumulative effects of many such lenslets can then be calculated through the matrix eigendecomposition theorem, where $\mathbf{P}$ is a matrix comprising the eigen*vectors* of $\mathbf{M}$ and $\mathbf{D}$ is a diagonal matrix comprising the eigen*values* of $\mathbf{M}$.

$$\mathbf{M^N} = \mathbf{MM...M} = (\mathbf{M})^N = \mathbf{PD^NP^{-1}} \tag{4}$$

The eigenvalues $E_\pm$, which are a complex conjugate pair if $4f > T$, may then be expressed as:

$$E_\pm = 1 - \frac{T}{2f} \pm i\frac{T}{2f}\sqrt{\frac{4f}{T} - 1} = a \pm ib = \exp\left(\pm i\varphi\right) \tag{5}$$

Where $\varphi$ is the phase angle of the complex eigenvalues, i.e.:

$$\varphi = \arctan\left(\frac{b}{a}\right) = \arctan\left(\frac{\sqrt{4fT - T^2}}{2f - T}\right) \tag{6}$$

By use of eq. 4 the expression for $\mathbf{M^N}$ then becomes

$$\begin{aligned}\mathbf{M^N} &= \begin{bmatrix} 1 & 1 \\ \frac{1}{if\sin\varphi} & \frac{-1}{if\sin\varphi} \end{bmatrix} \begin{bmatrix} \exp\left(-iN\varphi\right) & 0 \\ 0 & \exp\left(iN\varphi\right) \end{bmatrix} \begin{bmatrix} 1 & 1 \\ \frac{1}{if\sin\varphi} & \frac{-1}{if\sin\varphi} \end{bmatrix}^{-1} \\ &= \begin{bmatrix} \cos\left(N\varphi\right) & f\sin\left(\varphi\right)\sin\left(N\varphi\right) \\ \frac{-\sin\left(N\varphi\right)}{f\sin\left(\varphi\right)} & \cos\left(N\varphi\right) \end{bmatrix}\end{aligned} \tag{7}$$

We can then extract the focal length $f_N$ for the CRL (as measured from the CRL exit) from $\mathbf{M^N}$:

$$f_N = -\frac{\mathbf{M^N_{11}}}{\mathbf{M^N_{21}}} = f\sin\left(\varphi\right)\cot\left(N\varphi\right) \tag{8}$$

This approach is sufficiently general that other lens geometries can be described by re-calculating $\mathbf{M}$ and $\mathbf{M^N}$. This is demonstrated in the latter part of this document during the discussion of interdigitated lenslet geometries.

## C. Attenuation

The Beer-Lambert law describes the attenuation $\alpha$ of a ray passing through a 1D lens with linear absorption coefficient $\mu$ and local thickness $t$ at position $r$:

$$\alpha(r) = \exp\left[-\mu t(r)\right] \tag{9}$$

Individual lenslets are assumed to have a parabolic profile, meaning that the thickness as function of the radial position, $t(r)$ is given by:

$$t(r) = T_0 + \frac{r^2}{R} \tag{10}$$

Thus, neglecting the effects of air between lenslets, a single lenslet will attenuate the ray according to:

$$\alpha(r) = \exp\left(-\mu T_0\right) \times \exp\left(\frac{-\mu r^2}{R}\right) \tag{11}$$

The cumulative attenuation $\alpha_N(r)$ of a ray as it travels through $N$ lenslets is then the product of the individual attenuation contributions from each lenslet:

$$\alpha_N(r) = \prod_{n=1}^{N} \alpha(r_n) = \exp\left(-N\mu T_0\right) \times \exp\left(\frac{-\mu}{R}\sum_{n=1}^{N} r_n^2\right) \tag{12}$$

Assuming that a ray strikes the entry of the CRL at position $r_0$ and angle $w_0$, we calculate the position $r_n$ and angle $w_n$ of the ray at the longitudinal centre of each successive lenslet in the CRL, as per Fig. S2.

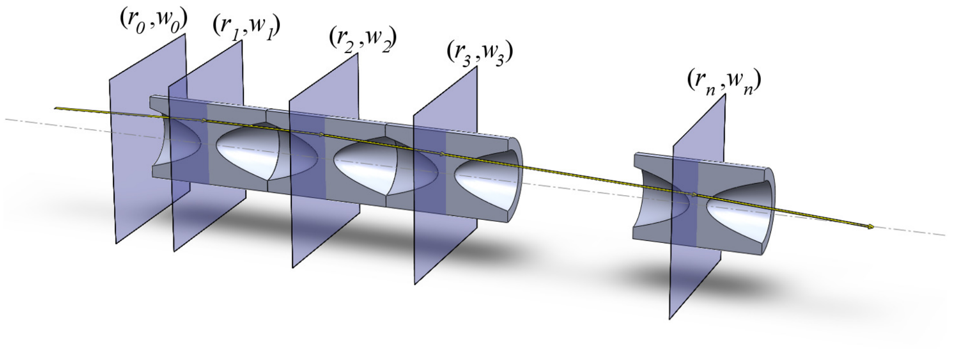


FIG. S2. Propagation geometry within the CRL. As the ray travels from left to right, it first strikes the CRL entry plane $(r_0, w_0)$ before propagating through the individual lens planes $(r_1, w_1)$ to $(r_n, w_n)$ at the $n^{th}$ lenslet.

We accomplish this by finding the position and angle at the exit of each (i.e. the $n^{th}$) lenslet, then back-propagating by half a lenslet thickness, $T/2$:

$$\begin{bmatrix} r_n \\ w_n \end{bmatrix} = \begin{bmatrix} 1 & -T/2 \\ 0 & 1 \end{bmatrix} \mathbf{M^n} \begin{bmatrix} r_0 \\ w_0 \end{bmatrix} \tag{13}$$

This gives the following expression for $r_n$, which is used extensively from here forth:

$$\begin{aligned} r_n &= \left(\mathbf{M^n_{11}} - \frac{T}{2}\mathbf{M^n_{21}}\right) r_0 + \left(\mathbf{M^n_{12}} - \frac{T}{2}\mathbf{M^n_{22}}\right) w_0 \\ &= \left[\cos(n\varphi) + \frac{T\sin(n\varphi)}{2f\sin(\varphi)}\right] r_0 + \left[f\sin(\varphi)\sin(n\varphi) - \frac{T}{2}\cos(n\varphi)\right] w_0 \end{aligned} \tag{14}$$

As we use the paraxial approximation, it is acceptable to assume that the true distance traversed within the lenslet profile is the same as if the ray were parallel with the optical axis. Thus, the local angle within the lens, $w_n$ is not needed in the analysis of absorption-related effects.

## D. Vignetting and angular acceptance

This formalism describes the optical performance of a full-field x-ray microscope in terms of the vignetting and angular acceptance functions. These functions are specific to the microscope configuration in Fig. S3, where a ray passes through three planes of interest: the sample plane ($r_s$,$w_s$), the objective entry plane ($r_0$,$w_0$) and the detector plane ($r_d$,$w_d$).

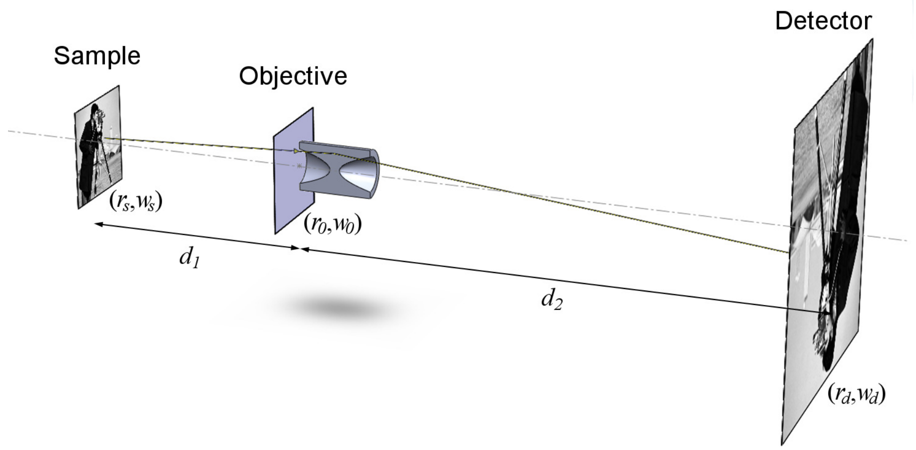


FIG. S3. Propagation geometry of a simple bright-field x-ray microscope. The ray travels from left to right, resulting in a magnified and inverted image of the sample on the detector plane.

In this configuration, the image magnification is given by $\mathcal{M}$ and the position $r_0$ and angle $w_0$ of the ray at the objective entry plane is related to the initial position $r_s$ and angle $w_s$ at the sample plane through the sample-objective distance $d_1$:

$$r_0 = r_s + d_1 w_s \tag{15}$$

$$w_0 = w_s \tag{16}$$

By substituting eqs. 15 and 16 into eq. 14 we then describe $r_n$ in terms of the sample plane coordinates $r_s$ and $w_s$:

$$r_n(w_s, r_s) = w_s \left[ d_1 \left( \mathbf{M^n_{11}} - \frac{T}{2}\mathbf{M^n_{21}} \right) + \mathbf{M^n_{12}} - \frac{T}{2}\mathbf{M^n_{22}} \right] + r_s \left( \mathbf{M^n_{11}} - \frac{T}{2}\mathbf{M^n_{21}} \right) \tag{17}$$

Recalling eq. 12, the cumulative attenuation $\alpha_N$ can then be rewritten in the followng form:

$$\alpha_N(r_s, w_s) = \exp\left(-N\mu T_0\right) \times \exp\left[-(A_N w_s^2 + B_N r_s w_s + C_N r_s^2)\right] \tag{18}$$

Where $A_N$, $B_N$ and $C_N$ are the coefficients:

$$A_N = \frac{\mu}{R} \sum_{n=1}^{N} \left[ d_1 \left( \mathbf{M^n_{11}} - \frac{T}{2}\mathbf{M^n_{21}} \right) + \left( \mathbf{M^n_{12}} - \frac{T}{2}\mathbf{M^n_{22}} \right) \right]^2 \tag{19}$$

$$B_N = \frac{2\mu}{R} \sum_{n=1}^{N} \left( \mathbf{M^n_{11}} - \frac{T}{2}\mathbf{M^n_{21}} \right) \left[ d_1 \left( \mathbf{M^n_{11}} - \frac{T}{2}\mathbf{M^n_{21}} \right) + \left( \mathbf{M^n_{12}} - \frac{T}{2}\mathbf{M^n_{22}} \right) \right] \tag{20}$$

$$C_N = \frac{\mu}{R} \sum_{n=1}^{N} \left( \mathbf{M^n_{11}} - \frac{T}{2}\mathbf{M^n_{21}} \right)^2 \tag{21}$$

The sums in these coefficients are geometric series and have analytical solutions, however for brevity we will not provide them here. The shape of the function $\alpha_N(r_s, w_s)$ is that of a tilted 2D Gaussian, shown in Fig. S4.

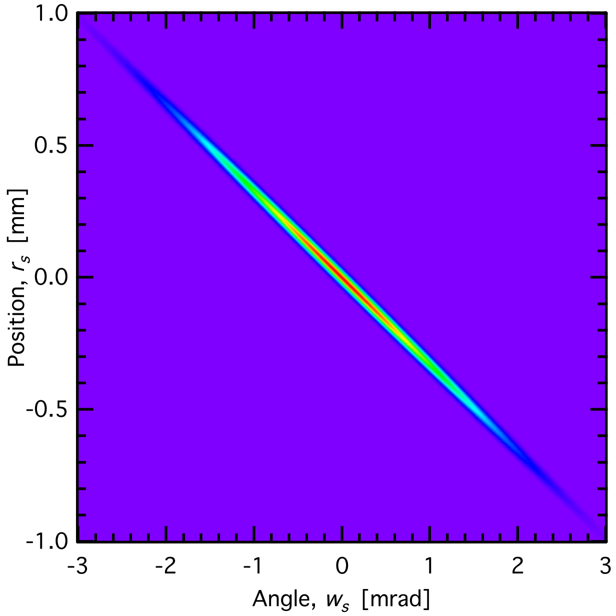


FIG. S4. Plot of eq. 18, showing attenuation $\alpha_N(r_s, w_s)$ as a function of position $r_s$ and angle $w_s$ on the sample plane. The plot corresponds to the 20 $\mu$m Si-based interdigitated CRL used in this study.

One can gain an immediate insight into the optical behaviour of the imaging system by rearranging $\alpha_N(r_s, w_s)$ in eq. 18:

$$\alpha_N(r_s, w_s) = \exp\left(-N\mu T_0\right) \times \exp\left[-\left(C_N - \frac{B_N^2}{4A_N}\right) r_s^2\right] \times \exp\left[-A_N(w_s + \frac{B_N}{2A_N} r_s)\right] \quad (22)$$

In this form, eq. 22 is clearly a product of a scaling coefficient and two Gaussian functions correponding to the *vignetting function*, which describes the reduction in brightness from the centre of the optical axis towards its periphery, and the *angular acceptance function*, which describes the angle over which the lens collects radiation emitted from a point $r_s$ on the sample plane.

The vignetting function is therefore expressed as:

$$I_v(r_s) = \exp\left(\frac{-r_s^2}{2\sigma_v^2}\right) \quad (23)$$

Which has the standard deviation $\sigma_v$:

$$\sigma_v = \sqrt{\frac{2A_N}{4A_N C_N - B_N^2}} \quad (24)$$

While the angular acceptance function is:

$$I_a(w_s, r_s) = \exp\left[\frac{-(w_s - \gamma r_s)^2}{2\sigma_a^2}\right] \tag{25}$$

Which has the standard deviation $\sigma_a$:

$$\sigma_a = \sqrt{\frac{1}{2A_N}} \tag{26}$$

And the offset $\gamma$:

$$\gamma = \frac{B_N}{2A_N} \tag{27}$$

These terms $\sigma_a$, $\sigma_v$ and $\gamma$ are invaluable for the characterisation, optimisation and comparison of CRL designs and configurations in the latter parts of this document and in the calculation of NA and $\sigma_a$ in Figs. 4 and 5 in the main text.

## E. Non-parallel incident wavefronts

The vignetting and angular acceptance functions in eqs. 23 and 25 pertain to the CRL alone and, while they are adequate for the optimization and comparison of CRL designs and configurations, they cannot be used for the prediction of experimentally-observed intensity distributions in their present form. Instead, we must account for the small size and divergence of the Gaussian x-ray source, which significantly modifies the intensity distribution of the x-rays scattered by the sample and thus affects the optical behaviour of the microscope. Here, we derive corrected functions for the angular acceptance,$\bar{\sigma_v}$ and vignetting,$\bar{\sigma_a}$ that account for the angular, spatial and intensity distribution of the incident x-rays.

We first consider an incident ray striking the sample plane at position $r_s$ at an angle $w_s'$ to the optical axis, and an outgoing (scattered) ray with an angle of $w_s$ to the optical axis. The angle between the incident and outgoing ray is then:

$$\Delta w_s = w_s - w_s' \tag{28}$$

In the case of a x-rays generated by an undulator or following conditioning by an absorption-limited CRL (e.g. a condenser), the incident wave field $I_0(r_s, w_s')$ is typically a 2D Gaussian, which we define here in terms of the coefficients $A_0$, $B_0$ and $C_0$:

$$I_0(r_s, w_s') = \exp\left[-(A_0 w_s'^2 + B_0 r_s w_s' + C_0 r_s^2)\right] \tag{29}$$

Thus, by rearranging and substituting eq. 28 into the expression for the attenuation $\alpha_N(r_s, w_s)$ (eq. 22), and multiplying this with $I_0(r_s, w_s')$, we can derive a function $I_{scatt}(r_s, \Delta w_s, w_s')$ for the intensity of the rays exiting the CRL according to their position on the sample plane $r_s$, scattering angle $\Delta w_s$ and incident angle $w_s'$:

$$\begin{aligned} I_{scatt}(r_s, \Delta w_s, w_s') &= \alpha_N(r_s, \Delta w_s + w_s') \times I_0(r_s, w_s') \\ &= \exp\left(-\mu N T_0\right) \\ &\times \exp\left\{-[A_N(\Delta w_s + w_s')^2 + B_N(\Delta w_s + w_s')r_s + C_N r_s^2]\right\} \\ &\times \exp\left[-(A_0 w_s'^2 + B_0 w_s' r_s + C_0 r_s^2)\right] \end{aligned} \tag{30}$$

Integrating over the incident ray angle $w_s'$ then gives:

$$\begin{aligned} I_{scatt}(r_s, \Delta w_s) &= \int_{-\infty}^{\infty} I_d(r_s, \Delta w, w_s')\, dw_s' \\ &= \frac{\exp\left(-N\mu T_0\right)\sqrt{\pi}}{\sqrt{A_N + A_0}} \\ &\times \exp\left\{-\left[\left(C_N - \frac{B_N^2}{4A_N}\right) + \left(C_0 - \frac{B_0^2}{4A_0}\right)\right] r_s^2\right\} \\ &\times \exp\left\{-\left(\frac{A_N A_0}{A_N + A_0}\right)\left[\Delta w_s + \left(\frac{B_N}{2A_N} - \frac{B_0}{2A_0}\right) r_s\right]^2\right\} \end{aligned} \tag{31}$$

As with eq. 22, the final equation for $I_{scatt}(r_s, \Delta w_s)$ is the product of a scaling coefficient and two Gaussian functions correponding to the vignetting and angular acceptance functions, albeit now accounting for the incident wavefront.

This vignetting function accounting for the source is then:

$$\begin{aligned} I_v(r_s) &= \exp\left\{-\left[\left(C_N - \frac{B_N^2}{4A_N}\right) + \left(C_0 - \frac{B_0^2}{4A_0}\right)\right] r_s^2\right\} \\ &= \exp\left(\frac{-r_s^2}{2\bar{\sigma_v}^2}\right) \end{aligned} \tag{32}$$

Which has the standard deviation $\bar{\sigma_v}$ given by:

$$\bar{\sigma_v} = \sqrt{\frac{2(A_N A_0)}{4A_N A_0(C_N + C_0) - (A_0 B_N^2 + A_N B_0^2)}} \tag{33}$$

And the angular acceptance function is:

$$
\begin{aligned}
I_a(\Delta w_s, r_s) &= \exp\left\{-\left(\frac{A_N A_0}{A_N + A_0}\right)\left[\Delta w_s + \left(\frac{B_N}{2A_N} - \frac{B_0}{2A_0}\right) r_s\right]^2\right\} \\
&= \exp\left\{\frac{[\Delta w_s - \bar{\gamma} r_s]^2}{2\bar{\sigma_a}^2}\right\}
\end{aligned}
\tag{34}
$$

Which has the standard standard deviation $\bar{\sigma_a}$ given by:

$$
\bar{\sigma_a} = \sqrt{\frac{1}{2A_N} + \frac{1}{2A_0}} \tag{35}
$$

And the offset function $\bar{\gamma}$:

$$
\bar{\gamma} = \frac{B_N}{2A_N} - \frac{B_0}{2A_0} \tag{36}
$$

Thus, we can see that the properties of the source wavefront play an important role in the intensity distribution and angular acceptance of the XRM. Of particular note is that effective NA can be increased via a highly divergent source (a result consistent with visible light microscopy).

It is also worth noting that in cases where the sample is only weakly absorbing (e.g. at the hard x-ray energies used here), the observed intensity distribution will include an additional (and possibly dominating) contribution to the vignetting function from the transmitted, unscattered x-rays. For example, consider the analysis of the flat-field image associated with Figs. 3 and 4 in the main text: calculating the value of $\sigma_v$ based on eq. 24 yields a value of 435 $\mu$m, compared to the experimentally determined values of $\approx 18.7$ $\mu$m. If we assume that the sample is close to transparent, then the intensity of these transmitted x-rays according to their position on the sample plane, $I_{trans}(r_s)$, can be calculated easily by assuming that $\Delta w_s = 0$. Then eq. 31 becomes:

$$
I_{trans}(r_s) = \frac{\exp(-N\mu T_0)\sqrt{\pi}}{\sqrt{A_N + A_0}} \times \exp\left\{-\left[(C_N + C_0) - \frac{(B_N + B_0)^2}{4(A_N + A_0)}\right] r_s^2\right\} \tag{37}
$$

This is another Gaussian function, which has a standard deviation $\bar{\sigma_v}$ of:

$$
\bar{\sigma_v} = \sqrt{\frac{2(A_N + A_0)}{4(A_N + A_0)(C_N + C_0) - (B_N + B_0)^2}} \tag{38}
$$

This is confirmed by the calculated value of $\bar{\sigma_v}$ for the experimental configuration of 18.5 $\mu$m, which is substantially closer to the measured value of 18.7 $\mu$m. This also shows that measurements of the flat-field vignetting function is a straightforward way to characterise imaging lenses (as demonstrated in the main text).

### F. Estimating resolution and depth-of-field

When the incident wave is either flat or a Gaussian with very low divergence (i.e. $A_0 \gg A_N$), we can consider it a Gaussian beam with with a waist $\omega_0$ and Rayleigh range $z_R$, defined in terms of the full-width at $e^{-2}$ of the maximum intensity (a standard practice in Gaussian beam optics)[1]:

$$\omega_0 = \frac{\lambda}{2\pi\sigma_a} \tag{39}$$

$$z_R = \frac{\lambda}{4\pi\sigma_a^2} \tag{40}$$

The depth of field (D.o.F.) can then be estimated since it is related to the Rayleigh range:

$$\text{D.o.F.} = 2z_R = \frac{\lambda}{2\pi\sigma_a^2} \tag{41}$$

While the NA is linearly proportional to the angular acceptance according to:

$$\text{NA} = \frac{\omega_0}{z_R} = 2\sigma_a \tag{42}$$

The spatial resolution of an imaging system is directly related to its NA, however in this case the 'tails' of the Gaussian angular acceptance function ($I_a$) contribute appreciably to the optical transfer function (OTF). This is discussed in detail in the latter part of this text, where it is shown that the maximum resolvable spatial frequency (i.e. best resolution) is ultimately determined by the extents of the Gaussian and thus the background noise and counting statistics present in the system. One can nonetheless make a reasonably accurate approximation of the spatial resolution at the sample plane ($\Delta r_s$) using the following relationship[6]:

$$\Delta r_s \approx \frac{0.75\lambda}{2\text{NA}} \tag{43}$$

## G. Optimisation

We have demonstrated that the parameters defining individual lenslets ($R$,$T$,$T_0$,$\delta/\mu$), their configuration within a CRL ($N$) and the imaging geometry ($d_1$,$\mathcal{M}$,$\lambda$) all contribute to the overall performance of a CRL-based XRM. However, it is not yet clear what values of these parameters maximise performance. The main purpose of the optimisation scheme presented here is to enable fair and direct comparison of lenslet geometries by comparing their *optimised* performance.

In establishing a figure-of-merit for the optimisation, we first consider the way in which an x-ray objective is used in an XRM. Experiments are typically carried out at single (or a limited range of) energies prescribed by the sample (e.g. to take advantage of contrast from attenuation, scattering or fluorescence) and at specific magnifications (e.g. to give a defined resolution or field-of-view). Thus, at a given energy and magnification, a high-performing lens will enable both high resolution (small $\Delta r_s$) while maximising the total intensity at the detector plane, $I_{tot}$, giving the figure-of-merit $\zeta$:

$$\zeta = \frac{I_{tot}}{\Delta r_s} \propto \mathrm{NA} \iint I_d(r_d, w_d)\, dw_d\, dr_d \tag{44}$$

Here, NA is defined in Eq. 42, while the integrated intensity $I_{tot}$ is a single number representing the efficiency over the field of view (FOV) of the sample. To derive this, we first note that the relationship between the position and angle of a ray at the sample and detector planes is given by:

$$r_s = \frac{r_d}{\mathcal{M}} \tag{45}$$

$$w_s = \mathcal{M} w_d - \mathbf{M^N_{21}} r_d \tag{46}$$

Making the simplification that the incident rays comprise a flat, parallel wavefront (i.e. $I_0$ is a constant), the intensity distribution at the detector plane is then:

$$I_d(r_d, w_d) = \frac{I_0}{\mathcal{M}^2} \times \alpha_N \left( \frac{r_d}{\mathcal{M}}, \mathcal{M} w_d - \mathbf{M^N_{21}} r_d \right) \tag{47}$$

The total intensity at the detector plane, $I_{tot}$ is then obtained by integrating $I_d(r_d, w_d)$ with respect to both the angles accepted by the objective (i.e. $r_s$), and the position across

the field of view (FOV) at the sample plane (i.e. $r_s$):

$$\begin{aligned} I_{tot} &= 2\int_0^{FOV/2}\int_{-\infty}^{\infty} I_d\left(\mathcal{M}r_s, \frac{w_s}{\mathcal{M}} + \mathbf{M_{21}^N} r_s\right)\, dw_s\, dr_s \\ &= \frac{2I_0\exp\left(-\mu N T_0\right)}{\mathcal{M}^2}\int_0^{FOV/2}\int_{-\infty}^{\infty}\exp\left[-(A_N w_s^2 + B_N w_s r_s C_N r_s^2)\right] dw_s\, dr_s \\ &= \frac{2\pi I_0\exp\left(-\mu N T_0\right)}{\mathcal{M}^2\sqrt{4A_N C_N - B_N^2}} \times \operatorname{erf}\left(\frac{FOV}{4}\sqrt{\frac{4A_N C_N - B_N^2}{A_N}}\right) \end{aligned} \tag{48}$$

Multiplying by NA and removing the constant prefactors then gives the figure of merit $\zeta$:

$$\zeta = \frac{\exp\left(-\mu N T_0\right)}{\sqrt{A_N(4A_N C_N - B_N^2)}} \times \operatorname{erf}\left(\frac{FOV}{4}\sqrt{\frac{4A_N C_N - B_N^2}{A_N}}\right) \tag{49}$$

Since we want to maximise $\zeta$, we then use numerical methods to find $N$ for which its derivative equals zero:

$$\frac{\partial \zeta}{\partial N} = 0 \tag{50}$$

Noting that the maximum number of lenslets is ultimately limited by the $\cot\left(N\varphi\right)$ term in eq. 8:

$$N_{max} = \frac{\pi}{\varphi} \tag{51}$$

At this point, it is relevant to discuss the differences between the figure-of-merit used in this work and those previously described in the literature[5,6]. The fact that a) different types of experiments have different requirements of the CRL, and b) the intensity distribution and resolution functions include terms specific to the experimental geometry emphasises that the figure-of-merit used to optimise a CRL depends intimately on its intended use. For example, a CRL used as condenser or conditioning optic will aim to produce the smallest possible spot size or highest gain (local intensification relative to the unperturbed beam), while an ideal imaging CRL maximises resolution and image intensity. As such, we avoid comparing the figure-of-merit used here to those pertaining to condensers.

In this work, the figure-of-merit assumes that the transmission and spatial resolution are equally important. Practically speaking, this is not always the case as there is typically

an upper limit to the image acquisition rate (e.g. due to the detector), implying a similar upper limit to the transmission of the lens. In such cases where the detector is prone to oversaturation it would be pragmatic to 'trade' the excess transmission for improved resolution, despite being at the cost of optical efficiency. Considering the incident beam flux, attenuation and detector characteristics in the figure-of-merit through appropriate weighting functions would therefore be of potential benefit in the optimisation of a CRL for specific experiments, but is outside the scope of this supporting document.

In determining the optimum number of lenses for a given energy, x-ray magnification and lenslet geometry, we now have a way of directly comparing the performance of different lenslet geometries (or the efficiency costs associated with changing the XRM configuration). It is by this method we generated Fig. 2 in the main article, which compares the NA (based on eqs. 26 and 42) and total integrated image intensity (from eq. 48) of various types of CRLs at hard x-ray energies. The calculations involved optimising the number of lenses using eq. 49, and assumed a constant x-ray magnification of 10 and a sample FOV of $200 \times 200$ $\mu$m, approximately consistent with a 2k×2k detector with a 1 $\mu$m pixel size. The specific materials and lenslet geometries used in the plot are given in Table 1.

TABLE I. Table of values used in Fig. 2 in the main article. * denotes the lens geometry of the prototype

| Lens material | Configuration | Radius $R$ [$\mu$m] | Aperture [$\mu$m] | Thickness $T$ [mm] | Web $T_0$ [$\mu$m] |
|---|---|---|---|---|---|
| Beryllium | axisymmetric | 50 | 631 | 2 | 10 |
| Aluminium | axisymmetric | 50 | 631 | 2 | 10 |
| PMMA | interdigitated | 10 | 76.8 | 1.2 | 10 |
| Silicon* | interdigitated | 20 | 294 | 2.95 | 20 |
| Silicon | interdigitated | 5 | 38.4 | 0.6 | 5 |

## H. Transfer functions

The optical performance of the x-ray microscope is described by the optical transfer function (OTF)[7]. To maintain consistency with the experimental results of the main paper, we here consider the scenario of an x-ray microscope with a diffraction-limited objective under incoherent illumination. As the RTM approach cannot explicitly account for coherency

and diffraction phenomena, we now use a Fourier optics approach.

The foundation of this analysis is the intensity convolution integral, which describes how the intensity impulse response $|h|^2$ affects the sample intensity distribution $I_s(r_s)$ to result in the image intensity distribution at the detector, $I_d(r_d)$.

$$I(r_d) = \int_{-\infty}^{\infty} |h(r_d - r_s)|^2 I(r_s)\, dr_s \tag{52}$$

This can be expressed in terms of the normalised frequency distributions of $I_s(r_s)$ and $I_d(r_d)$, denoted here as $G_s(f_R)$ and $G_d(f_R)$, respectively.

$$G_d(f_R) = \mathcal{H}(f_R) G_s(f_R) \tag{53}$$

Here, $\mathcal{H}(f_R)$ is the OTF, which is related to the intensity impulse response $|h|^2$ according to:

$$\mathcal{H}(f_R) = \frac{\mathcal{F}|h|^2}{\int_{-\infty}^{\infty} |h(r_d)|^2\, dr_d} \tag{54}$$

Where $\mathcal{F}|h|^2$ denotes the Fourier transform of $|h|^2$.

We can then express the intensity distributions at the sample and detector planes through the OTF:

$$I_d(r_d) = \mathcal{F}^{-1}|\mathcal{H}(f_R)|^2 \otimes I_s(r_s) \tag{55}$$

In the case of an aberration-free system (which we assume here), the OTF is described in terms of the pupil function, which defines the spatial acceptance of light by the objective. This is directly related to the angular acceptance function $I_a(w_s, r_s)$ through the relationship: $r_0 = d_1 w_s + r_s$. Thus, recalling the angular acceptance function in eq. 34 (note that this incorporates the effects of the source wavefront!), we state the OTF as follows:

$$\begin{aligned} \mathcal{H}(f_R) &= \frac{\int_{-\infty}^{\infty} I_a\left(\frac{r_0 - r_s}{d_1} + \frac{\lambda f_R}{2}, r_s\right) I_a\left(\frac{r_0 - r_s}{d_1} - \frac{\lambda f_R}{2}, r_s\right) dr_0}{\int_{-\infty}^{\infty} I_a\left(\frac{r_0 - r_s}{d_1}, r_s\right)^2 dr_0} \\ &= \exp\left(\frac{-f_R^2 \lambda^2}{4\bar{\sigma_a}^2}\right) \end{aligned} \tag{56}$$

$\mathcal{H}$ is therefore a Gaussian function in the spatial frequency domain whose shape is independent of $r_s$, implying that the optical performance remains constant over the image field of view.

The squared magnitude of the OTF is the modulation transfer function (MTF), which describes the contrast response of the system across the spatial frequency domain. The resolution of the system is therefore related to the maximum spatial frequency where there is a measurable modulation/contrast (referred to as the cutoff frequency, $f_0$):

$$\Delta r_s = \frac{1}{f_0} \tag{57}$$

In optical systems where the pupil function is well-defined (e.g. a pinhole), the MTF function is triangular[7]. However, in Gaussian cases such as ours, $f_0$ extends asymptotically in the 'tails' of the function. Yet, a well-defined cutoff frequency can be observed when there is background noise in the system (which is always present in real XRMs), as $f_0$ is the frequency at which the MTF intersects the background function. This implies that the resolution can be improved by increasing the counting statistics and reducing the background noise in the system (e.g., through detectors with high dynamic range).

## I. Extending the RTM approach to misaligned interdigitated lenses

In considering true 2D optical systems such as interdigitated or misaligned lenses, the $2 \times 2$ ray-transfer matrix notation outlined previously is no longer sufficient and a $4 \times 4$ notation must be used to account for the differences between the horizontal and vertical optical properties[1]. The $4 \times 4$ formalism must include the position and angle in both the horizontal $(x, u)$ and vertical $(y, v)$ directions. While this increases the complexity of the calculations, the overall process is largely identical to the 1D case.

$$\begin{bmatrix} x_1 \\ u_1 \\ y_1 \\ v_1 \end{bmatrix} = \mathbf{M} \begin{bmatrix} x_0 \\ u_0 \\ y_0 \\ v_0 \end{bmatrix} \tag{58}$$

One of the key capabilities of the extended RTM notation - and the primary reason it is used here - is that it can account for misalignments between refractive elements[1]. In the case

of the interdigitated geometry described in this paper (Fig S5), it is essential to understand the effect of non-perpendicularity of the lenses and to quantify any astigmatism that may result.

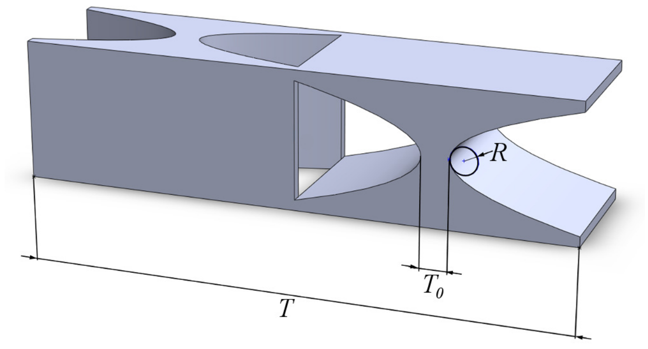


FIG. S5. Geometry of the interdigitated 2D lenslet used in this work

We here consider the simplified case where the horizontal and vertical focusing elements are spatially coincident and located in the centre of the 2D lenslet, but are misaligned longitudinally by $2\theta$. In incorporating the rotational misalignment, we apply the rotation matrix $\mathbf{R}$ to each refracting component individually, resulting in the RTM for the lenslet:

$$\mathbf{M} = \mathbf{S}(T/2)\left[\mathbf{R^T}(\theta)\mathbf{L}(-1/f,0)\mathbf{R}(\theta)\right]\left[\mathbf{R^T}(-\theta)\mathbf{L}(0,-1/f)\mathbf{R}(-\theta)\right]\mathbf{S}(T/2) \tag{59}$$

Where $\mathbf{S}$ is the propagation matrix, $\mathbf{L}$ is the refractive matrix and $\mathbf{R}$ is the rotation matrix accounting for the misalignment of the lenslets. These are defined as follows:

$$\mathbf{S}(d) = \begin{bmatrix} 1 & d & 0 & 0 \\ 0 & 1 & 0 & 0 \\ 0 & 0 & 1 & d \\ 0 & 0 & 0 & 1 \end{bmatrix} \tag{60}$$

$$\mathbf{L}(P_1, P_2) = \begin{bmatrix} 1 & 0 & 0 & 0 \\ P_1 & 1 & 0 & 0 \\ 0 & 0 & 1 & 0 \\ 0 & 0 & P_2 & 1 \end{bmatrix} \tag{61}$$

$$\mathbf{R}(\theta) = \begin{bmatrix} \cos\left(\frac{\pi}{4}+\theta\right) & 0 & \sin\left(\frac{\pi}{4}+\theta\right) & 0 \\ 0 & \cos\left(\frac{\pi}{4}+\theta\right) & 0 & \sin\left(\frac{\pi}{4}+\theta\right) \\ -\sin\left(\frac{\pi}{4}+\theta\right) & 0 & \cos\left(\frac{\pi}{4}+\theta\right) & 0 \\ 0 & -\sin\left(\frac{\pi}{4}+\theta\right) & 0 & \cos\left(\frac{\pi}{4}+\theta\right) \end{bmatrix} \tag{62}$$

We note that the rotation matrix includes a shift of 45°, meaning that the axes of the lenses in $\mathbf{M}$ are now at 45°with respect to horizontal and vertical. The reason for this is purely mathematical, as it creates a block-diagonal matrix that can be manipulated much more straightforwardly:

$$\mathbf{M} = \begin{bmatrix} 1-\frac{T}{2f}[1-\sin(2\theta)] & T-\frac{T^2}{4f}[1-\sin(2\theta)] & 0 & 0 \\ \frac{-1}{f}[1-\sin(2\theta)] & 1-\frac{T}{2f}[1-\sin(2\theta)] & 0 & 0 \\ 0 & 0 & 1-\frac{T}{2f}[1+\sin(2\theta)] & T-\frac{T^2}{4f}[1+\sin(2\theta)] \\ 0 & 0 & \frac{-1}{f}[1+\sin(2\theta)] & 1-\frac{T}{2f}[1+\sin(2\theta)] \end{bmatrix} \tag{63}$$

One can see by inspection that the two $2\times 2$ submatrices correspond to the two perpendicular directions, and that their respective terms differ by the factor $1\pm\sin 2\theta$. Nonetheless, we note that the matrix $\mathbf{M}$ has the complex eigenvalues characterised by the phase angles $\varphi_1$ and $\varphi_2$:

$$\begin{aligned} E_{1\pm} &= 1-\frac{T}{2f}[1-\sin(2\theta)] \pm \frac{i}{2f}\sqrt{T[1-\sin(2\theta)](4f-T[1-\sin(2\theta)])} = \exp(\pm i\varphi_1) \\ E_{2\pm} &= 1-\frac{T}{2f}[1+\sin(2\theta)] \pm \frac{i}{2f}\sqrt{T[1+\sin(2\theta)](4f-T[1+\sin(2\theta)])} = \exp(\pm i\varphi_2) \end{aligned} \tag{64}$$

Carrying out the exponentiation of $\mathbf{M}$ yields a full $4\times 4$ matrix representing the misaligned 2D lens with N pairs of lenslets.

$$\mathbf{M}^N = \begin{bmatrix} \cos(N\varphi_1) & f\frac{\sin(N\varphi_1)\sin(\varphi_1)}{1-\sin(2\theta)} & 0 & 0 \\ -\frac{[1-\sin(2\theta)]\sin(N\varphi_1)}{f\sin(\varphi_1)} & \cos(N\varphi_1) & 0 & 0 \\ 0 & 0 & \cos(N\varphi_2) & f\frac{\sin(N\varphi_2)\sin(\varphi_2)}{1+\sin(2\theta)} \\ 0 & 0 & -\frac{[1+\sin(2\theta)]\sin(N\varphi_2)}{f\sin(\varphi_2)} & \cos(N\varphi_2) \end{bmatrix} \tag{65}$$

The resulting focal lengths are then extracted as:

$$f_1 = -\frac{\mathbf{M^N_{11}}}{\mathbf{M^N_{21}}} = \frac{f\sin(\varphi_1)}{\tan(N\varphi_1)[1-\sin(2\theta)]} \simeq \frac{f}{N[1-\sin(2\theta)]}$$
$$f_2 = -\frac{\mathbf{M^N_{33}}}{\mathbf{M^N_{43}}} = \frac{f\sin(\varphi_2)}{\tan(N\varphi_2)[1+\sin(2\theta)]} \simeq \frac{f}{N[1+\sin(2\theta)]} \quad (66)$$

The approximation is valid for $N\varphi_1$ and $N\varphi_2 \ll 1$, i.e. $f \gg NT$. Thus, the difference in focal length (i.e. astigmatism) in an interdigitated lens is:

$$\Delta f = f_1 - f_2 \simeq \frac{2f\sin(2\theta)}{N\cos^2(2\theta)} \approx 4\theta\frac{f}{N} \quad (67)$$

## II. MANUFACTURING AND EXPERIMENTAL DETAILS

### A. Manufacturing

The prototype interdigitated lens was manufactured at DTU Danchip, the cleanroom facility at the Technical University of Denmark. It comprises two individual silicon CRLs arranged orthogonally on a steel gauge block using a micromanipulator and an optical microscope and glued in place (Fig. S6).

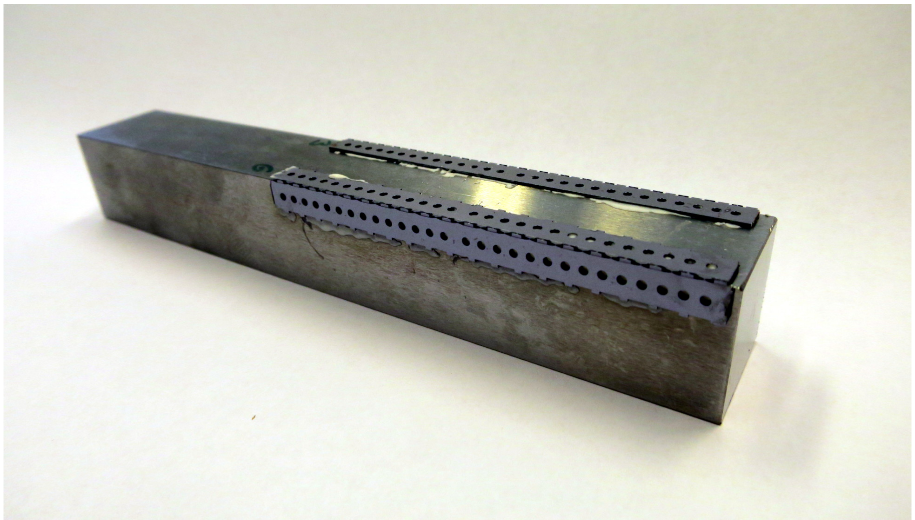

FIG. S6. Photograph of interdigitated Si 2D lens. For reference, the steel guage block is $16 \times 16 \times 110$mm$^3$.

The individual chips contained 20 lenslets, each of which were 1 mm long, 350 $\mu$m wide, 350 $\mu$m deep, had a nominal radius of curvature of 20 $\mu$m, a web thickness of 10 $\mu$m, and

were separated 100 $\mu$m from each other in the direction of the x-ray beam. The starting material was a 4-inch silicon wafer with a thickness of 350 $\mu$m. The manufacture included contact UV-lithography and pattern transfer by reactive ion etching into a 50 nm thick aluminium oxide layer deposited by atomic layer deposition, which served as a hard mask for subsequent deep reactive ion etching (DRIE) of the silicon. In addition, we performed a surface smoothening step by the thermal growth of a 3 $\mu$m thick silicon oxide layer followed by its removal in buffered hydrofluoric acid. Individual chips containing the CRLs of 1 cm width and 7 cm length were separated from the rest of the wafer using a micro machining tool equipped with a picosecond pulsed solid state laser.

Assembled lenses were inspected by scanning electron microscopy and atomic force microscopy (AFM)[8]. Fitting of the AFM data presented in the paper enabled confirmation of the true ROC of the lenses and the accuracy of these as 20.5026 ±0.0164 $\mu$m.

### B. Experiment

The hard x-ray microscope was configured at ID06 of the European Synchrotron. It comprised a set of tungsten slits, the sample, the interdigitated x-ray lens and a detector in the configuration shown in Fig. S7. All components were mounted on a common granite bench to minimise vibration and mechanical instability.

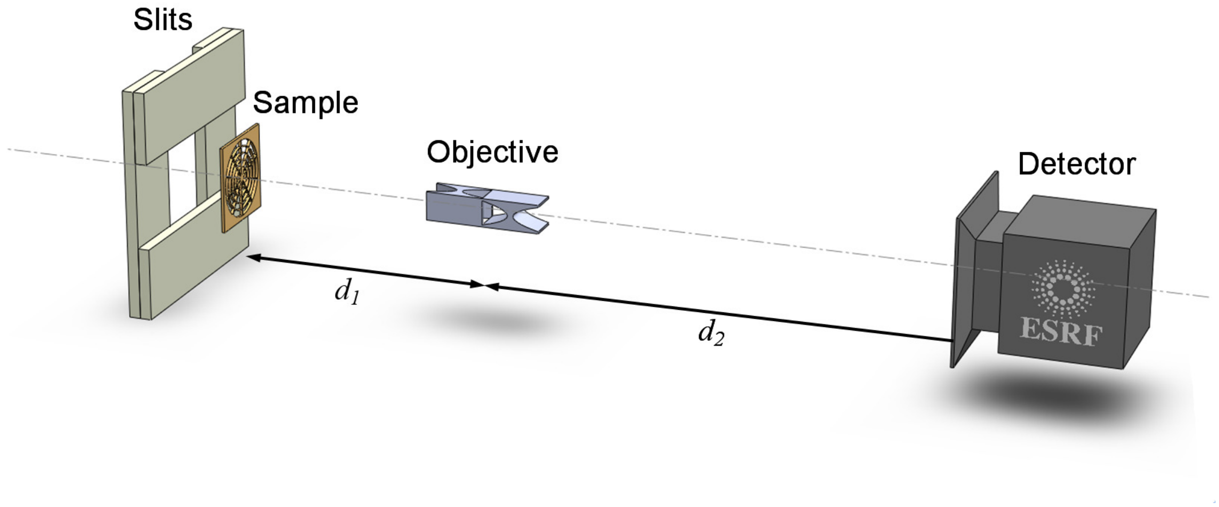


FIG. S7. Schematic of the experimental geometry used to test the interdigitated objective

X-rays of 17 keV (±10 eV) were selected by a Si (111) double-bounce monochromator

located 38 m from the source. To generate an incoherent secondary source, a rotating amorphous carbon disc was inserted 58 m from the source (2 m upstream of the sample).

The sample was an XRESO-50HC resolution chart (NTT-AT, Japan) containing a selection of different features with sizes varying from 4 $\mu$m to 50 nm. It was located 10 cm downstream from the slits, which were 60 m from the source and configured with a $200 \times 200$ $\mu$m square aperture

The interdigitated objective (see above for detailed specifications) was positioned in the imaging configuration $d_1 = 378.9$ mm from the sample and $d_1 + d_2 = 3921.1$ mm from the detector, giving a magnification of 10.35 over a 4.3 m distance. Alignment of the objective was a straightforward process involving coupled translation and rotational scans to maximise the transmission measured on a photodiode.

The detector was a high-resolution Sensicam QE (PCO, Germany): a 12-bit CCD with $1376 \times 1040$ pixels of $6.45 \times 6.45$ $\mu$m size. A $10\times$ microscope objective and 10 $\mu$m LAG:Eu scintillator were fitted, resulting in a 0.645 $\mu$m pixel size and a 0.887 x 0.671 mm$^2$ field of view.

## REFERENCES


[1]N. Hodgson and H. Weber, in *Laser Resonators and Beam Propagation SE - 2*, Springer Series in Optical Sciences, Vol. 108 (Springer New York, 2005) Chap. Geometrica, pp. 7–55.

[2]V. V. Protopopov and K. A. Valiev, Optics Communications **151**, 297 (1998).

[3]R. H. Pantell, J. Feinstein, H. R. Beguiristain, M. A. Piestrup, C. K. Gary, and J. T. Cremer, Applied Optics **42**, 719 (2003).

[4]C. G. Schroer and B. Lengeler, Physical Review Letters **94**, 54802 (2005).

[5]S. Poulsen and H. Poulsen, Metallurgical and Materials Transactions A **45**, 4772 (2014).

[6]B. Lengeler, C. Schroer, J. Tümmler, B. Benner, M. Richwin, A. Snigirev, I. Snigireva, and M. Drakopoulos, Journal of Synchrotron Radiation **6**, 1153 (1999).

[7]J. W. Goodman, *Introduction to Fourier optics*, Vol. 2 (McGraw-hill New York, 1968).

[8]F. Stöhr, J. Michael-Lindhard, H. Simons, H. F. Poulsen, J. Hübner, O. Hansen, J. Garnaes, and F. Jensen, Microelectronic Engineering **141**, 6 (2015).
